# Supplementary material for: FlowDCN: Exploring DCN-like Architectures for Fast Image Generation with Arbitrary Resolution
Source: arXiv:2410.22655 source file (2024-10-30)
Supplement: Supplementary file 1 [file supp2.tex]

\section*{D. ~More Uncurated $256\times256$ Samples Visualization}
% \begin{table}[H]
%     \centering
%     \renewcommand{\arraystretch}{0.}
%     \setlength{\tabcolsep}{1pt}
%     \begin{tabular}{m{.5cm}m{15cm}}
%     % \begin{tabularx}{\textwidth}{X{5}X{50}X{50}}
%     ID & {\hspace{5.5cm} $256\times256$~Random Samples} \\
%     \rotatebox{90}{4} &  \includegraphics[width=0.95\linewidth]{article/figures/seeds_out/4.png} \\
%     \rotatebox{90}{5} &  \includegraphics[width=0.95\linewidth]{article/figures/seeds_out/5.png} \\
%     \rotatebox{90}{22} &  \includegraphics[width=0.95\linewidth]{article/figures/seeds_out/22.png} \\
%     \rotatebox{90}{30} &  \includegraphics[width=0.95\linewidth]{article/figures/seeds_out/30.png} \\
    
%     \end{tabular}
%     \label{tab:256_images}
% \end{table}

\begin{table}[H]
    \centering
    
    \setlength{\tabcolsep}{1pt}
    \begin{tabular}{m{.5cm}m{15cm}}
    % \begin{tabularx}{\textwidth}{X{5}X{50}X{50}}
    ID & {\hspace{5.5cm} $256\times256$~Random Samples} \\
    \rotatebox{90}{4} &  \includegraphics[width=0.95\linewidth]{article/figures/seeds_out/4.png} \\
    \rotatebox{90}{5} &  \includegraphics[width=0.95\linewidth]{article/figures/seeds_out/5.png} \\
    \rotatebox{90}{22} &  \includegraphics[width=0.95\linewidth]{article/figures/seeds_out/22.png} \\
    \rotatebox{90}{30} &  \includegraphics[width=0.95\linewidth]{article/figures/seeds_out/30.png} \\
    \rotatebox{90}{33} &  \includegraphics[width=0.95\linewidth]{article/figures/seeds_out/33.png} \\
    \rotatebox{90}{59} &  \includegraphics[width=0.95\linewidth]{article/figures/seeds_out/59.png} \\
    \rotatebox{90}{64} &  \includegraphics[width=0.95\linewidth]{article/figures/seeds_out/64.png} \\
    \rotatebox{90}{69} &  \includegraphics[width=0.95\linewidth]{article/figures/seeds_out/69.png} \\
    % \rotatebox{90}{70} &  \includegraphics[width=0.95\linewidth]{article/figures/seeds_out/70.png} \\
    \rotatebox{90}{88} &  \includegraphics[width=0.95\linewidth]{article/figures/seeds_out/88.png} \\
    \rotatebox{90}{89} &  \includegraphics[width=0.95\linewidth]{article/figures/seeds_out/89.png} \\
    \rotatebox{90}{107} &  \includegraphics[width=0.95\linewidth]{article/figures/seeds_out/107.png} \\
    \rotatebox{90}{118} &  \includegraphics[width=0.95\linewidth]{article/figures/seeds_out/118.png} \\
    \rotatebox{90}{120} &  \includegraphics[width=0.95\linewidth]{article/figures/seeds_out/120.png} \\
    \rotatebox{90}{130} &  \includegraphics[width=0.95\linewidth]{article/figures/seeds_out/130.png} \\
    \rotatebox{90}{71} &  \includegraphics[width=0.95\linewidth]{article/figures/seeds_out/71.png} \\
    % \rotatebox{90}{72} &  \includegraphics[width=0.95\linewidth]{article/figures/seeds_out/72.png} \\
    \rotatebox{90}{355} &  \includegraphics[width=0.95\linewidth]{article/figures/seeds_out/355.png} \\
    % \rotatebox{90}{76} &  \includegraphics[width=0.95\linewidth]{article/figures/seeds_out/76.png} \\
    % \rotatebox{90}{77} &  \includegraphics[width=0.95\linewidth]{article/figures/seeds_out/77.png} \\
    % \rotatebox{90}{148} &  \includegraphics[width=0.95\linewidth]{article/figures/seeds_out/148.png} \\
    \end{tabular}
    \label{tab:256_images}
\end{table}

\begin{table}[H]
    \centering
    
    \setlength{\tabcolsep}{1pt}
    \begin{tabular}{m{.5cm}m{15cm}}
    % \begin{tabularx}{\textwidth}{X{5}X{50}X{50}}
    ID & {\hspace{5.5cm} $256\times256$~Random Samples} \\
    \rotatebox{90}{74} &  \includegraphics[width=0.95\linewidth]{article/figures/seeds_out/74.png} \\
    \rotatebox{90}{429} &  \includegraphics[width=0.95\linewidth]{article/figures/seeds_out/429.png} \\
    \rotatebox{90}{207} &  \includegraphics[width=0.95\linewidth]{article/figures/seeds_out/207.png} \\
    \rotatebox{90}{277} &  \includegraphics[width=0.95\linewidth]{article/figures/seeds_out/277.png} \\
    \rotatebox{90}{279} &  \includegraphics[width=0.95\linewidth]{article/figures/seeds_out/279.png} \\
    % \rotatebox{90}{282} &  \includegraphics[width=0.95\linewidth]{article/figures/seeds_out/282.png} \\
    \rotatebox{90}{291} &  \includegraphics[width=0.95\linewidth]{article/figures/seeds_out/291.png} \\
    % \rotatebox{90}{73} &  \includegraphics[width=0.95\linewidth]{article/figures/seeds_out/73.png} \\
    \rotatebox{90}{360} &  \includegraphics[width=0.95\linewidth]{article/figures/seeds_out/360.png} \\
    \rotatebox{90}{387} &  \includegraphics[width=0.95\linewidth]{article/figures/seeds_out/387.png} \\
    \rotatebox{90}{388} &  \includegraphics[width=0.95\linewidth]{article/figures/seeds_out/388.png} \\
    \rotatebox{90}{397} &  \includegraphics[width=0.95\linewidth]{article/figures/seeds_out/397.png} \\
    \rotatebox{90}{417} &  \includegraphics[width=0.95\linewidth]{article/figures/seeds_out/417.png} \\
    \rotatebox{90}{944} &  \includegraphics[width=0.95\linewidth]{article/figures/seeds_out/944.png} \\
    \rotatebox{90}{971} &  \includegraphics[width=0.95\linewidth]{article/figures/seeds_out/971.png} \\
    \rotatebox{90}{972} &  \includegraphics[width=0.95\linewidth]{article/figures/seeds_out/972.png} \\
    \rotatebox{90}{980} &  \includegraphics[width=0.95\linewidth]{article/figures/seeds_out/980.png} \\
    \rotatebox{90}{985} &  \includegraphics[width=0.95\linewidth]{article/figures/seeds_out/985.png} \\
    \end{tabular}
    \label{tab:256_images}
\end{table}

\newpage
\section*{E. ~Fewer Steps Uncurated ODE Samples $256\times256$ Compared to SiT}
\begin{table}[H]
    \centering
    
    \begin{tabular}{cl}
    % \begin{tabularx}{\textwidth}{X{5}X{50}X{50}}
    & {\small ODE Solver Steps $\rightarrow$ \hspace{1.2em}  3 \hspace{3em} 4 \hspace{3.2em} 5 \hspace{3.2em} 6 \hspace{3.2em} 7 \hspace{3.2em} 8 \hspace{3.2em} 9 \hspace{3.2em} 10} \\
    \rotatebox{90}{\small SiT} & 
    \includegraphics[width=0.95\linewidth]{article/figures/sit_traj/2_1.png} \\
    \rotatebox{90}{\small Ours} & 
    \includegraphics[width=0.95\linewidth]{article/figures/flowdcn_traj/2_1.png} \\
    \rotatebox{90}{\small SiT} & 
    \includegraphics[width=0.95\linewidth]{article/figures/sit_traj/5_0.png} \\
    \rotatebox{90}{\small Ours} & 
    \includegraphics[width=0.95\linewidth]{article/figures/flowdcn_traj/5_0.png} \\
    \rotatebox{90}{\small SiT} & 
    \includegraphics[width=0.95\linewidth]{article/figures/sit_traj/88_1.png} \\
    \rotatebox{90}{\small Ours} & 
    \includegraphics[width=0.95\linewidth]{article/figures/flowdcn_traj/88_1.png} \\
    \rotatebox{90}{\small SiT} & 
    \includegraphics[width=0.95\linewidth]{article/figures/sit_traj/88_2.png} \\
    \rotatebox{90}{\small Ours} & 
    \includegraphics[width=0.95\linewidth]{article/figures/flowdcn_traj/88_2.png} \\
    \rotatebox{90}{\small SiT} & 
    \includegraphics[width=0.95\linewidth]{article/figures/sit_traj/89_2.png} \\
    \rotatebox{90}{\small Ours} & 
    \includegraphics[width=0.95\linewidth]{article/figures/flowdcn_traj/89_2.png} \\
    \rotatebox{90}{\small SiT} & 
    \includegraphics[width=0.95\linewidth]{article/figures/sit_traj/89_1.png} \\
    \rotatebox{90}{\small Ours} & 
    \includegraphics[width=0.95\linewidth]{article/figures/flowdcn_traj/89_1.png} \\
    \rotatebox{90}{\small SiT} & 
    \includegraphics[width=0.95\linewidth]{article/figures/sit_traj/120_0.png} \\
    \rotatebox{90}{\small Ours} & 
    \includegraphics[width=0.95\linewidth]{article/figures/flowdcn_traj/120_0.png} \\ 
    \rotatebox{90}{\small SiT} & 
    \includegraphics[width=0.95\linewidth]{article/figures/sit_traj/120_2.png} \\
    \rotatebox{90}{\small Ours} & 
    \includegraphics[width=0.95\linewidth]{article/figures/flowdcn_traj/120_2.png} \\
    \end{tabular}
    \label{tab:app_odes1}
\end{table}

\begin{table}[H]
    \centering
    
    \begin{tabular}{cl}
    % \begin{tabularx}{\textwidth}{X{5}X{50}X{50}}
    & {\small ODE Solver Steps $\rightarrow$ \hspace{1.2em}  3 \hspace{3em} 4 \hspace{3.2em} 5 \hspace{3.2em} 6 \hspace{3.2em} 7 \hspace{3.2em} 8 \hspace{3.2em} 9 \hspace{3.2em} 10} \\
    \rotatebox{90}{\small SiT} & 
    \includegraphics[width=0.95\linewidth]{article/figures/sit_traj/207_0.png} \\
    \rotatebox{90}{\small Ours} & 
    \includegraphics[width=0.95\linewidth]{article/figures/flowdcn_traj/207_0.png} \\
    \rotatebox{90}{\small SiT} & 
    \includegraphics[width=0.95\linewidth]{article/figures/sit_traj/207_1.png} \\
    \rotatebox{90}{\small Ours} & 
    \includegraphics[width=0.95\linewidth]{article/figures/flowdcn_traj/207_1.png} \\

    \rotatebox{90}{\small SiT} & 
    \includegraphics[width=0.95\linewidth]{article/figures/sit_traj/360_0.png} \\
    \rotatebox{90}{\small Ours} & 
    \includegraphics[width=0.95\linewidth]{article/figures/flowdcn_traj/360_0.png} \\
    \rotatebox{90}{\small SiT} & 
    \includegraphics[width=0.95\linewidth]{article/figures/sit_traj/360_1.png} \\
    \rotatebox{90}{\small Ours} & 
    \includegraphics[width=0.95\linewidth]{article/figures/flowdcn_traj/360_1.png} \\

    \rotatebox{90}{\small SiT} & 
    \includegraphics[width=0.95\linewidth]{article/figures/sit_traj/387_2.png} \\
    \rotatebox{90}{\small Ours} & 
    \includegraphics[width=0.95\linewidth]{article/figures/flowdcn_traj/387_2.png} \\
    \rotatebox{90}{\small SiT} & 
    \includegraphics[width=0.95\linewidth]{article/figures/sit_traj/387_3.png} \\
    \rotatebox{90}{\small Ours} & 
    \includegraphics[width=0.95\linewidth]{article/figures/flowdcn_traj/387_3.png} \\

    \rotatebox{90}{\small SiT} & 
    \includegraphics[width=0.95\linewidth]{article/figures/sit_traj/388_1.png} \\
    \rotatebox{90}{\small Ours} & 
    \includegraphics[width=0.95\linewidth]{article/figures/flowdcn_traj/388_1.png} \\
    \rotatebox{90}{\small SiT} & 
    \includegraphics[width=0.95\linewidth]{article/figures/sit_traj/417_0.png} \\
    \rotatebox{90}{\small Ours} & 
    \includegraphics[width=0.95\linewidth]{article/figures/flowdcn_traj/417_0.png} \\
    \end{tabular}
    \label{tab:app_odes3}
\end{table}

\begin{table}[H]
    \centering
    
    \begin{tabular}{cl}
    % \begin{tabularx}{\textwidth}{X{5}X{50}X{50}}
    & {\small ODE Solver Steps $\rightarrow$ \hspace{1.2em}  3 \hspace{3em} 4 \hspace{3.2em} 5 \hspace{3.2em} 6 \hspace{3.2em} 7 \hspace{3.2em} 8 \hspace{3.2em} 9 \hspace{3.2em} 10} \\
    \rotatebox{90}{\small SiT} & 
    \includegraphics[width=0.95\linewidth]{article/figures/sit_traj/417_1.png} \\
    \rotatebox{90}{\small Ours} & 
    \includegraphics[width=0.95\linewidth]{article/figures/flowdcn_traj/417_1.png} \\
    \rotatebox{90}{\small SiT} & 
    \includegraphics[width=0.95\linewidth]{article/figures/sit_traj/944_0.png} \\
    \rotatebox{90}{\small Ours} & 
    \includegraphics[width=0.95\linewidth]{article/figures/flowdcn_traj/944_0.png} \\
    \rotatebox{90}{\small SiT} & 
    \includegraphics[width=0.95\linewidth]{article/figures/sit_traj/944_2.png} \\
    \rotatebox{90}{\small Ours} & 
    \includegraphics[width=0.95\linewidth]{article/figures/flowdcn_traj/944_2.png} \\

    \rotatebox{90}{\small SiT} & 
    \includegraphics[width=0.95\linewidth]{article/figures/sit_traj/971_0.png} \\
    \rotatebox{90}{\small Ours} & 
    \includegraphics[width=0.95\linewidth]{article/figures/flowdcn_traj/971_0.png} \\
    \rotatebox{90}{\small SiT} & 
    \includegraphics[width=0.95\linewidth]{article/figures/sit_traj/971_2.png} \\
    \rotatebox{90}{\small Ours} & 
    \includegraphics[width=0.95\linewidth]{article/figures/flowdcn_traj/971_2.png} \\

    \rotatebox{90}{\small SiT} & 
    \includegraphics[width=0.95\linewidth]{article/figures/sit_traj/980_0.png} \\
    \rotatebox{90}{\small Ours} & 
    \includegraphics[width=0.95\linewidth]{article/figures/flowdcn_traj/980_0.png} \\
    \rotatebox{90}{\small SiT} & 
    \includegraphics[width=0.95\linewidth]{article/figures/sit_traj/980_1.png} \\
    \rotatebox{90}{\small Ours} & 
    \includegraphics[width=0.95\linewidth]{article/figures/flowdcn_traj/980_1.png} \\

    \rotatebox{90}{\small SiT} & 
    \includegraphics[width=0.95\linewidth]{article/figures/sit_traj/33_0.png} \\
    \rotatebox{90}{\small Ours} & 
    \includegraphics[width=0.95\linewidth]{article/figures/flowdcn_traj/33_0.png} \\
    % \rotatebox{90}{\small SiT} & 
    % \includegraphics[width=0.95\linewidth]{article/figures/sit_traj/33_3.png} \\
    % \rotatebox{90}{\small Ours} & 
    % \includegraphics[width=0.95\linewidth]{article/figures/flowdcn_traj/33_3.png} \\
    \end{tabular}
    \label{tab:app_odes2}
\end{table}

\newpage
\section*{F. ~Wide Images Samples {\small ($256\times 1024$)}}
\begin{figure}[H]
    \centering
    \includegraphics[width=0.95\linewidth]{article/figures/long_images/longimage_972.pdf}
    \includegraphics[width=0.95\linewidth]{article/figures/long_images/longimage_980.pdf}
    \includegraphics[width=0.95\linewidth]{article/figures/long_images/longimage_437.pdf}
    \caption{Wide images examples of Class ID ($972$ , $980$, $437$)}
    \label{fig:long_images}
\end{figure}

\section*{G. ~More Uncarted Samples with $S_\text{max}$ Adjustment ~{\small ($512\times 256$ and $256\times512$) }}

\begin{table}[H]
    \centering
   \setlength{\tabcolsep}{1pt}
    \begin{tabular}{m{.5cm}m{6cm}m{6cm}m{.01cm}}
    % \begin{tabularx}{\textwidth}{X{5}X{50}X{50}}
        & \centering with $S_\text{max}$ Adjustment & 
          \centering without $S_\text{max}$ Adjustment & \\
         \rotatebox{90}{107} & 
         \includegraphics[width=1.0\linewidth]{article/figures/wabs_hv/107.png} & \includegraphics[width=1.0\linewidth]{article/figures/woabs_hv/107.png}  \\
         % \rotatebox{90}{3} & 
         % \includegraphics[width=1.0\linewidth]{article/figures/wabs_hv/3.png} & \includegraphics[width=1.0\linewidth]{article/figures/woabs_hv/3.png}  \\
         \rotatebox{90}{5} & 
         \includegraphics[width=1.0\linewidth]{article/figures/wabs_hv/5.png} & \includegraphics[width=1.0\linewidth]{article/figures/woabs_hv/5.png}  \\
         % \rotatebox{90}{30} & 
         % \includegraphics[width=1.0\linewidth]{article/figures/wabs_hv/30.png} & \includegraphics[width=1.0\linewidth]{article/figures/woabs_hv/30.png}  \\
         \rotatebox{90}{88} & 
         \includegraphics[width=1.0\linewidth]{article/figures/wabs_hv/88.png} & \includegraphics[width=1.0\linewidth]{article/figures/woabs_hv/88.png}  \\
         \rotatebox{90}{89} & 
         \includegraphics[width=1.0\linewidth]{article/figures/wabs_hv/89.png} & \includegraphics[width=1.0\linewidth]{article/figures/woabs_hv/89.png}  \\
    \end{tabular}
    
    \label{tab:app_abs}
\end{table}

\begin{table}[H]
    \centering
   \setlength{\tabcolsep}{1pt}
    \begin{tabular}{m{.5cm}m{6cm}m{6cm}m{.01cm}}
    % \begin{tabularx}{\textwidth}{X{5}X{50}X{50}}
        & \centering with $S_\text{max}$ Adjustment & 
          \centering without $S_\text{max}$ Adjustment & \\
         % \rotatebox{90}{130} & 
         % \includegraphics[width=1.0\linewidth]{article/figures/wabs_hv/130.png} & \includegraphics[width=1.0\linewidth]{article/figures/woabs_hv/130.png}  \\
         % \rotatebox{90}{148} & 
         % \includegraphics[width=1.0\linewidth]{article/figures/wabs_hv/148.png} & \includegraphics[width=1.0\linewidth]{article/figures/woabs_hv/148.png}  \\
         % \rotatebox{90}{277} & 
         % \includegraphics[width=1.0\linewidth]{article/figures/wabs_hv/277.png} & \includegraphics[width=1.0\linewidth]{article/figures/woabs_hv/277.png}  \\
         % \rotatebox{90}{279} & 
         % \includegraphics[width=1.0\linewidth]{article/figures/wabs_hv/279.png} & \includegraphics[width=1.0\linewidth]{article/figures/woabs_hv/279.png}  \\
         % \rotatebox{90}{282} & 
         % \includegraphics[width=1.0\linewidth]{article/figures/wabs_hv/282.png} & \includegraphics[width=1.0\linewidth]{article/figures/woabs_hv/282.png}  \\
         \rotatebox{90}{355} & 
         \includegraphics[width=1.0\linewidth]{article/figures/wabs_hv/355.png} & \includegraphics[width=1.0\linewidth]{article/figures/woabs_hv/355.png}  \\
         \rotatebox{90}{360} & 
         \includegraphics[width=1.0\linewidth]{article/figures/wabs_hv/360.png} & \includegraphics[width=1.0\linewidth]{article/figures/woabs_hv/360.png}  \\
         \rotatebox{90}{397} & 
         \includegraphics[width=1.0\linewidth]{article/figures/wabs_hv/397.png} & \includegraphics[width=1.0\linewidth]{article/figures/woabs_hv/397.png}  \\
         \rotatebox{90}{417} & 
         \includegraphics[width=1.0\linewidth]{article/figures/wabs_hv/417.png} & \includegraphics[width=1.0\linewidth]{article/figures/woabs_hv/417.png}  \\
         % \rotatebox{90}{971} & 
         % \includegraphics[width=1.0\linewidth]{article/figures/wabs_hv/971.png} & \includegraphics[width=1.0\linewidth]{article/figures/woabs_hv/971.png}  \\
    \end{tabular}
    
    \label{tab:app_abs3}
\end{table}

% \begin{table}[h]
%     \centering
%    \setlength{\tabcolsep}{1pt}
%     \begin{tabular}{m{.5cm}m{6cm}m{6cm}m{.01cm}}
%     % \begin{tabularx}{\textwidth}{X{5}X{50}X{50}}
%         & \centering with $S_\text{max}$ Adjustment & 
%           \centering without $S_\text{max}$ Adjustment & \\
%          % \rotatebox{90}{291} & 
%          % \includegraphics[width=1.0\linewidth]{article/figures/wabs_hv/291.png} & \includegraphics[width=1.0\linewidth]{article/figures/woabs_hv/291.png}  \\
%          % \rotatebox{90}{387} & 
%          % \includegraphics[width=1.0\linewidth]{article/figures/wabs_hv/387.png} & \includegraphics[width=1.0\linewidth]{article/figures/woabs_hv/387.png}  \\
         
%     \end{tabular}
    
%     \label{tab:app_abs4}
% \end{table}

% \begin{table}[h]
%     \centering
%    \setlength{\tabcolsep}{1pt}
%     \begin{tabular}{m{.5cm}m{6cm}m{6cm}m{.01cm}}
%     % \begin{tabularx}{\textwidth}{X{5}X{50}X{50}}
%         & \centering with $S_\text{max}$ Adjustment & 
%           \centering without $S_\text{max}$ Adjustment & \\
%          % \rotatebox{90}{388} & 
%          % \includegraphics[width=1.0\linewidth]{article/figures/wabs_hv/388.png} & \includegraphics[width=1.0\linewidth]{article/figures/woabs_hv/388.png}  \\
         
%          \rotatebox{90}{944} & 
%          \includegraphics[width=1.0\linewidth]{article/figures/wabs_hv/944.png} & \includegraphics[width=1.0\linewidth]{article/figures/woabs_hv/944.png}  \\

%     \end{tabular}
    
%     \label{tab:app_abs5}
% \end{table}
